# Supplementary material for: L$_0$onie: Compressing COINs with L$_0$-constraints
Source: arXiv:2207.04144 source file (2022-07-08)
Supplement: Supplementary file 1 [file mp_comparison_imagenet_APPENDIX.tex]

\begin{table}[h!]
\small
\centering

\caption{Sparse ResNet50 models on ImageNet. Structured $L_1$ magnitude pruning corresponds to the method of \citet{li2017l1pruning}, discarding the filters with the $(1 - \epsilon)$ lowest $L_1$-norms. ``Fine-tuning'' for zero epochs means \textit{no} fine-tuning. This table complements the results shown in Table \ref{tab:mp_comparison_imagenet}.}

\label{tab:mp_comparison_imagenet_APPENDIX}
\vspace{1ex}

\resizebox{\textwidth}{!}{%
\begin{tabular}{ccccccccc}
\hline
\multirow{2}{*}{\textbf{Target}} & \multirow{3}{*}{\textbf{Method}}  & \multirow{2}{*}{$L_0$-\textbf{density}} & \multirow{2}{*}{\textbf{Params}} & \multirow{2}{*}{\textbf{MACs}} & \multicolumn{4}{c}{\textbf{Val. Error} (\%)} \\
\cline{6-9}
\multirow{2}{*}{\textbf{Density}} & & \multirow{2}{*}{(\%)} & \multirow{2}{*}{(\%)} & \multirow{2}{*}{(\%)} &  \multicolumn{4}{c}{After fine-tuning for \# epochs} \\
& & & & & 0 & 1 & 10 & 20 \\
\hline
\hline
  \multirow{2}{*}{$-$} & \multirow{2}{*}{Pre-trained Baseline} & \multirow{2}{*}{$100$} & \multirow{2}{*}{[25.5M]}  & \multirow{2}{*}{[$4.12 \cdot 10^9$]}  & {\multirow{2}{*}{$23.90$}} & \multicolumn{3}{c}{\multirow{2}{*}{{\color{gray} --------------}}} \\
  & & & & & & & \\
 \hline
\multirow{6}{*}{$\epsilon = 90 \%$} & Constrained & \multirow{2}{*}{$90.51$} & \multirow{2}{*}{$87.96$} & \multirow{2}{*}{$85.68$} & {\multirow{2}{*}{$26.41$}} & \multicolumn{3}{c}{\multirow{2}{*}{{\color{gray} --------------}}} \\
& {\color{gray} \textit{Model-wise}} & & & & & & & \\
\cline{2-9}
& Constrained & \multirow{2}{*}{$90.51$} & \multirow{2}{*}{$88.00$} & \multirow{2}{*}{$86.98$} & {\multirow{2}{*}{$26.56$}} & \multicolumn{3}{c}{\multirow{2}{*}{{\color{gray} --------------}}} \\
& {\color{gray} \textit{Layer-wise}} & & & & & & & \\
\cline{2-9}
 & L1 - Mag. Prune & \multirow{2}{*}{$-$} & \multirow{2}{*}{$85.94$} & \multirow{2}{*}{$84.99$} & \multirow{2}{*}{$38.74$} & \multirow{2}{*}{$25.38$} & \multirow{2}{*}{$24.69$} &\multirow{2}{*}{$24.68$} \\
 & {\color{gray} \textit{Layer-wise}} & & & & & & & \\
\hline
\multirow{6}{*}{$\epsilon = 80 \%$} & Constrained & \multirow{2}{*}{$80.52$} & \multirow{2}{*}{$74.76$} & \multirow{2}{*}{$77.05$} & {\multirow{2}{*}{$27.56$}} & \multicolumn{3}{c}{\multirow{2}{*}{{\color{gray} --------------}}} \\
& {\color{gray} \textit{Model-wise}} & & & & & & & \\
\cline{2-9}
& Constrained & \multirow{2}{*}{$80.54$} & \multirow{2}{*}{$74.39$} & \multirow{2}{*}{$72.69$} & {\multirow{2}{*}{$27.86$}} & \multicolumn{3}{c}{\multirow{2}{*}{{\color{gray} --------------}}}\\
& {\color{gray} \textit{Layer-wise}} & & & & & & & \\
\cline{2-9}
& L1 - Mag. Prune & \multirow{2}{*}{$-$} & \multirow{2}{*}{$73.35$} & \multirow{2}{*}{$71.69$} & \multirow{2}{*}{$77.69$} & \multirow{2}{*}{$27.00$} & \multirow{2}{*}{$25.51$} & \multirow{2}{*}{$25.24$} \\
& {\color{gray} \textit{Layer-wise}} & & & & & & & \\
\hline
\multirow{6}{*}{$\epsilon = 70 \%$} & Constrained & \multirow{2}{*}{$70.40$} & \multirow{2}{*}{$62.38$} & \multirow{2}{*}{$68.16$} & {\multirow{2}{*}{$27.60$}} & \multicolumn{3}{c}{\multirow{2}{*}{{\color{gray} --------------}}} \\
& {\color{gray} \textit{Model-wise}} & & & & & & & \\
\cline{2-9}
& Constrained & \multirow{2}{*}{$70.73$} & \multirow{2}{*}{$61.09$} & \multirow{2}{*}{$57.72$} & {\multirow{2}{*}{$27.81$}} & \multicolumn{3}{c}{\multirow{2}{*}{{\color{gray} --------------}}} \\
& {\color{gray} \textit{Layer-wise}} & & & & & & & \\
\cline{2-9}
& L1 - Mag. Prune & \multirow{2}{*}{$-$} & \multirow{2}{*}{$62.15$} & \multirow{2}{*}{$59.85$} & \multirow{2}{*}{$97.78$} & \multirow{2}{*}{$29.04$} & \multirow{2}{*}{$26.80$} & \multirow{2}{*}{$26.14$} \\
& {\color{gray} \textit{Layer-wise}} & & & & & & & \\
\hline
\end{tabular}
}
\end{table}
