# Supplementary material for: L$_0$onie: Compressing COINs with L$_0$-constraints
Source: arXiv:2207.04144 source file (2022-07-08)
Supplement: Supplementary file 3 [file tiny_imagenet_APPENDIX_comparison.tex]

\begin{figure}[h!]
\setlength\tabcolsep{0pt}%
\hspace{-1.5cm}
\centering
\begin{tabular}{llccc}
 \centering
 & \hspace{2mm} & \hspace{-2mm} \textbf{$L_0$-density} & \hspace{6mm}\textbf{Parameters} & \hspace{5mm} \textbf{MACs} \\
 
\rotatebox{90}{\hspace{1.3cm} \textbf{Layer-wise}} & & \includegraphics[width=0.4\textwidth, trim={0mm 0mm 0mm 0mm}, clip]{figs/control/tiny_imagenet/L0ResNet18_layerwise.pdf}
 & \includegraphics[width=0.32\textwidth]{figs/error_vs_params/tiny_imagenet/L0ResNet18_layerwise.pdf}
 & \includegraphics[width=0.32\textwidth]{figs/error_vs_macs/tiny_imagenet/L0ResNet18_layerwise.pdf} \\
\rotatebox{90}{\hspace{1.3cm} \textbf{Model-wise}} &  & \includegraphics[width=0.4\textwidth, trim={0mm 0mm 0mm 0mm}, clip]{figs/control/tiny_imagenet/L0ResNet18_modelwise.pdf}
 & \includegraphics[width=0.32\textwidth]{figs/error_vs_params/tiny_imagenet/L0ResNet18_modelwise.pdf}
 & \includegraphics[width=0.32\textwidth]{figs/error_vs_macs/tiny_imagenet/L0ResNet18_modelwise.pdf} \\
\end{tabular}
    \caption[]{Training sparse ResNet18 models on TinyImageNet. {\small  This figure is the same as \cref{fig:tiny_imagenet_comparison}. We repeat it here for the reader's convenience.}}
    \label{fig:tiny_imagenet_APPENDIX_comparison}
\end{figure}
