# Supplementary material for: L$_0$onie: Compressing COINs with L$_0$-constraints
Source: arXiv:2207.04144 source file (2022-07-08)
Supplement: Supplementary file 4 [file mnist_table_APPENDIX.tex]

\begin{table*}[h!]

    \centering

    \caption{Achieved density levels and performance for sparse MLP and LeNet5 models     trained on MNIST for 200 epochs. Metrics aggregated over 5 runs. {\small $^\dag$Results by \citet{louizos2017learning} with $N$ representing the training set size (see \cref{app:normalized_l0}). This table is the same as \cref{tab:mnist}. We repeat it here for the reader's convenience.}}
    \label{tab:mnist_APPENDIX}
    \vspace{1ex}
    
    \resizebox{\textwidth}{!}{%
    \begin{tabular}{ccclccc}
      \hline
      \multirow{3}{*}{\textbf{Architecture}} & \multirow{3}{*}{\textbf{Grouping}} & \multirow{3}{*}{\textbf{Method}}  & \multirow{3}{*}{\textbf{\hspace{5mm}Hyper-parameters}} & \textbf{Pruned} & \multicolumn{2}{c}{\textbf{Val. Error} (\%)}  \\
      \cline{6-7} & & &  &  \multirow{2}{*}{\textbf{architecture}} & \multirow{2}{*}{best} & at 200 epochs \\
       & & & & &  & avg {\color{gray} $\pm$ 95\% CI}\\
      \hline
      \hline
       & \multirow{2}{*}{Model} & Pen.  &  $^\dag\lambda_{pen} = 0.1/N$ &  219-214-100 & 1.4 & --\\
       MLP & & Const. &  $\epsilon = 33 \%$ &  198-233-100 & 1.36 & 1.77 {\color{gray} $\pm$ 0.08}\\
       \cline{2-7}
       784-300-100 & \multirow{2}{*}{Layer} & Pen. &  $^\dag\lambda_{pen} = [0.1,0.1,0.1]/N$ &  266-88-33 & 1.8 & -- \\
      & & Const. &  $\epsilon = [30 \%, 30\%, 30\%]$ &  243-89-29 & 1.58 & 2.19 {\color{gray} $\pm$ 0.12 }\\
       \hline
       & \multirow{2}{*}{Model} & Pen. &   $^\dag\lambda_{pen} = 0.1/N$ &  20-25-45-462 & 0.9 & --\\
       LeNet5 & & Const. &  $\epsilon = 10\%$ &  20-21-34-407 & 0.56 & 1.01 {\color{gray} $\pm$ 0.05}\\
       \cline{2-7}
       20-50-800-500 & \multirow{2}{*}{Layer} & Pen. &  $^\dag\lambda_{pen} = [10,0.5,0.1,0.1]/N$ &  9-18-65-25 & 1.0 & -- \\
       & & Const. &  $\epsilon = [50\%, 30\%, 70\%, 10\%]$ &  10-14-224-29 & 0.7 & 0.91 {\color{gray} $\pm$ 0.05}\\
       \hline
    \end{tabular}
    } %

\end{table*}
